# Supplementary material for: On-the-Fly Ab Initio Hagedorn Wavepacket Dynamics: Single Vibronic Level Fluorescence Spectra of Difluorocarbene
Source: arXiv:2409.01862 source file (2024-12-16)
Supplement: Supplementary file 1 [file svl_lha_ab_initio_suppl_v03.pdf]

# Supplemental Material to On-the-Fly *Ab Initio* Hagedorn Wavepacket Dynamics: Single Vibronic Level Fluorescence Spectra of Difluorocarbene

Zhan Tong Zhang, Máté Visegrádi, and Jiří Vaníček

*Laboratory of Theoretical Physical Chemistry,*

*Institut des Sciences et Ingénierie Chimiques,*

*Ecole Polytechnique Fédérale de Lausanne (EPFL), CH-1015 Lausanne, Switzerland*

## I. OPTIMIZED GEOMETRIES AND FREQUENCIES OF THE $\tilde{X}^1A_1$ AND $\tilde{A}^1B_1$ STATES OF $CF_2$

The equilibrium geometries (r: C-F bond length; $\theta$: C-F-C bond angle) of the ground $\tilde{X}^1A_1$ and first excited $\tilde{A}^1B_1$ electronic states and the corresponding vibrational frequencies were calculated using the PBE0 functional and the aug-cc-pVTZ basis set. The computed values are compared to the experimental data [1–3] (as summarized in Ref. [4]) in Table I.

| $\tilde{X}^1A_1$ | r/Å | $\theta$/ deg | $\omega_1$/cm$^{-1}$ | $\omega_2$/cm$^{-1}$ | $\omega_3$/cm$^{-1}$ |
|---|---|---|---|---|---|
| PBE0/aug-cc-pVTZ | 1.2965 | 104.77 | 1255.43 | 680.61 | 1151.23 |
| Expt | 1.2975 | 104.81 | 1275.08 | 666.25 | 1114.44 |

(a) Ground electronic state

| $\tilde{A}^1B_1$ | r/Å | $\theta$/ deg | $\omega_1$/cm$^{-1}$ | $\omega_2$/cm$^{-1}$ | $\omega_3$/cm$^{-1}$ |
|---|---|---|---|---|---|
| TD-PBE0/aug-cc-pVTZ | 1.3054 | 123.27 | 1109.14 | 500.84 | 1362.81 |
| Expt | 1.316 | 122.3 | 1011 | 496 | 1180 |

(b) Excited electronic state

TABLE I: Geometries of $CF_2$ optimized at PBE0/aug-cc-pVTZ level of theory and the fundamental vibrational frequencies; for comparison, the experimentally (Expt) derived values are also shown.

## II. PROCEDURE USED TO SHIFT AND SCALE THE SVL EMISSION SPECTRA

Because the error in the electronic excitation energy obtained from electronic structure calculations is larger than the vibrational spacing in the spectra, a horizontal shift is applied to the computed spectra. Determining this shift correctly is crucial because the shift fixes the "zero" of frequency and therefore affects the frequency-dependent $\omega^3$ factor in Eq. (5), which is applied to the "wavepacket" spectra obtained by the Fourier transform of the autocorrelation function.

For each initial vibrational level $K$ of the excited electronic state, we applied the following procedure to the computed SVL fluorescence spectrum:

**Step 1**: The computed spectrum is horizontally shifted to account for the error in the electronic excitation energy obtained from electronic structure calculations. This shift determines the $\tilde{\nu}_{\text{em}}$ of the computed spectrum.

— In the adiabatic harmonic model, where the $2_0^K$ transition (i.e., the transition to the vibrational ground level of the electronic ground state) is well-defined and clearly visible, the computed spectrum is shifted such that its $2_0^K$ peak aligns with the $2_0^K$ peak in the experimental spectrum.

— In the vertical and local harmonic cases, the computed spectrum is shifted such that its highest peak aligns with the highest peak in the experimental spectrum. Note: When multiple SVL spectra are obtained from the same ab initio trajectory, their shifts should be approximately the same. In particular, the differences between the shifts should be much smaller than the vibrational spacing between the peaks. If a shift for one SVL differs substantially from others, the alignment for that SVL should be adjusted by the vibrational spacing. See below for an example in the local harmonic $2^2$ spectrum of $CF_2$.

**Step 2**: The spectrum computed by a Fourier transform of the autocorrelation function is multiplied by $\tilde{\nu}_{\text{em}}^3$ (since $\tilde{\nu}_{\text{em}} \propto \omega$ and the intensities will be normalized in the next step).

— In the vertical and local harmonic cases only, one needs to check the following: If, after applying the $\tilde{\nu}_{\text{em}}^3$ factor, the highest peak in the computed spectrum changes, the horizontal shift is revised such that the highest peak (after multiplication) is aligned to the highest experimental peak and Step 2 is repeated until the spectrum scaled by $\tilde{\nu}_{\text{em}}^3$ converges.

**Step 3**: The intensity of the highest peak is set to 1 in both computed and experimental spectra.

### A. Example of the adjustment in Step 1

In the $2^2$ local harmonic spectra of $CF_2$ (see Figs. 1 and 2 of the main text), the two highest peaks are neighboring each other and have similar intensities. The shift determined by matching the highest peaks produced a spectrum that appeared to be one vibrational quantum off from the experimental reference. This situation can be detected automatically and rigorously by a general procedure, which we demonstrate on our example of $2^2$ local harmonic spectra of $CF_2$:

We noticed that the shift determined in Step 1 for the $2^2$ spectrum was quite different (by approximately one vibrational quantum, $\sim 650$ cm$^{-1}$) from the shifts determined for other spectra obtained from the same trajectory:

| Initial vibrational excitation | Difference from average shift (determined by highest peak) (cm$^{-1}$) |
|---|---|
| $2^0$ | $-170$ |
| $2^1$ | $-125$ |
| $2^2$ | 553 |
| $2^3$ | $-105$ |
| $2^4$ | $-65$ |
| $2^5$ | $-50$ |
| $2^6$ | $-40$ |

We thus decided to shift the highest peak of the computed $2^2$ spectrum to align with the second-highest peak in the experiment. The shifts for all spectra are consistent after this adjustment:

| Initial vibrational excitation | Difference from average shift (determined by highest peak) (cm$^{-1}$) |
|---|---|
| $2^0$ | $-74$ |
| $2^1$ | $-29$ |
| $2^2$ | $-24$ |
| $2^3$ | $-9$ |
| $2^4$ | 31 |
| $2^5$ | 46 |
| $2^6$ | 56 |

This suggests that the alignments of all SVL spectra are correct and, indeed, the computed

$2^2$ spectrum now matches the experimental one better.


[1] F. Comes and D. Ramsay, J. Mol. Spec. **113**, 495 (1985).

[2] M. R. Cameron, S. H. Kable, and G. B. Bacskay, J. Chem. Phys. **103**, 4476 (1995).

[3] L. Margulès, J. Demaison, and J. E. Boggs, J. Phys. Chem. A **103**, 7632 (1999).

[4] F.-T. Chau, J. M. Dyke, E. P. F. Lee, and D. K. W. Mok, J. Chem. Phys. **115**, 5816 (2001).
